# Supplementary material for: Silver-Epoxy Microwave Filters and Thermalizers for Millikelvin Experiments
Source: arXiv:1403.6205 ancillary file (2014-03-25)
Supplement: Supplementary file 1 [file SOM.pdf]

Supplementary Information

# Silver-Epoxy Microwave Filters and Thermalizers for Millikelvin Experiments

Christian P. Scheller,[1] Sarah Heizmann,[1] Kristine Bedner,[1] Dominic Giss,[1] Matthias Meschke,[2] Dominik M. Zumbühl,[1,*] Jeramy D. Zimmerman,[3] and Arthur C. Gossard[3]

[1] *University of Basel, Klingelbergstrasse 82, CH-4056 Basel, Switzerland*

[2] *Low Temperature Lab, Aalto University, School of Science, 00076 Aalto, Finland*

[3] *Materials Department, University of California, Santa Barbara, CA93106, USA*

The attenuation of a coaxial cable can be calculated by means of transmission line theory[1], which extends the description of discrete electronic components to distributed elements. For a coaxial cable with resistance $R_{\mathrm{tot}}$ [Ω/m], given by the sum of inner and outer conductor resistance $R_{\mathrm{IC}}$ and $R_{\mathrm{OC}}$, with inductance $L$ [H/m], capacitance $C$ [F/m] and shunt conductance $G$ [S/m] (note that all parameters are per length), the attenuation in units of decibel as a function of frequency $\nu$ reads:

$$\text{Attenuation}(\nu) = 20 \log \left| e^{-\gamma z} \right|, \qquad \gamma = \sqrt{(R_{\mathrm{tot}} + 2\pi i \nu L)(G + 2\pi i \nu C)} \tag{1}$$

Here, $z$ denotes the wire length in units of m. Parameters $R_{\mathrm{tot}}$, $L$, $C$ and $G$ may be calculated from geometric dimensions of the coaxial cable (inner conductor diameter $D$, thickness $d_{\mathrm{Ins.}}$ of the polyurethane insulation and $d_{\mathrm{epoxy}}$ for the epoxy outer conductor), and material properties such as the dielectric constant $\epsilon_{\mathrm{Ins.}}$ of the polyurethane insulation and the conductivity $\sigma_{\mathrm{Cu}}$, $\sigma_{\mathrm{epoxy}}$, $\sigma_{\mathrm{Ins.}}$ of inner conductor, outer conductor and the insulator, respectively:

$$\begin{aligned}
R_{\mathrm{tot}} &= R_{\mathrm{IC}} + R_{\mathrm{OC}} = \frac{1}{\sigma_{\mathrm{Cu}} \left(\frac{D}{2}\right)^2 \pi} + \frac{1}{\sigma_{\mathrm{epoxy}} \left( \left(\frac{D}{2} + d_{\mathrm{Ins.}} + d_{\mathrm{epoxy}}\right)^2 - \left(\frac{D}{2} + d_{\mathrm{Ins.}}\right)^2 \right) \pi} \\
C &= \frac{2\pi \epsilon_0 \epsilon_{\mathrm{Ins.}}}{\ln\left(\frac{D/2 + d_{\mathrm{Ins.}}}{D/2}\right)} \\
L &= \frac{\mu_{\mathrm{Ins.}}}{2\pi} \ln\left(\frac{D/2 + d_{\mathrm{Ins.}}}{D/2}\right) \\
G &= \frac{\sigma_{\mathrm{Ins.}}}{\epsilon_{\mathrm{Ins.}}} C
\end{aligned} \tag{2}$$

As discussed in the main text, the skin effect forces AC currents to the conductor surface i.e. the skin depth $\delta_{\mathrm{Cu}} = 1/\sqrt{\sigma_{\mathrm{Cu}} \mu_{\mathrm{Cu}} \nu \pi}$ in case of copper and $\delta_{\mathrm{epoxy}} = 1/\sqrt{\sigma_{\mathrm{epoxy}} \mu_{\mathrm{epoxy}} \nu \pi}$ for the epoxy outer conductor (the permeabilities $\mu_{\mathrm{Cu}}$, $\mu_{\mathrm{epoxy}}$ and $\mu_{\mathrm{Ins.}}$ are assumed to be equal to the vacuum permeability $\mu_0$, since all those materials, copper and Ag-epoxy and polyurethane, are not magnetic). As a consequence, the resistance is modified to:

$$\begin{aligned}
R_{\mathrm{IC}}(\nu) &= \frac{1}{\sigma_{\mathrm{Cu}} \cdot \left( \left(\frac{D}{2}\right)^2 - \left(\frac{D}{2} - \delta_1\right)^2 \right)}, \qquad \delta_1 = \min(\delta_{\mathrm{Cu}}, D/2) \\
R_{\mathrm{OC}}(\nu) &= \frac{1}{\sigma_{\mathrm{epoxy}} \cdot \left( \left(\frac{D}{2} + d_{\mathrm{Ins.}} + \delta_2\right)^2 - \left(\frac{D}{2} + d_{\mathrm{Ins.}}\right)^2 \right)}, \qquad \delta_2 = \min(\delta_{\mathrm{epoxy}}, d_{\mathrm{epoxy}})
\end{aligned} \tag{3}$$

Note that eq. 3 gives an approxiated solution for $R_{\mathrm{IC}}(\nu)$ that is, however, very close to the exact solution which can be expressed in terms of bessel functions.

Next, experimental results are compared with attenuation curves obtained from transmission line theory, i.e. using eq. 1 ($C$, $L$ and $G$ are calculated from eq. 2 and the frequency dependent resistance is given in eq. 3). Fig. S1 shows the measured attenuation profile for a microwave filter with $z = 1.51\,\mathrm{m}$ of copper wire, a total DC resistance and capacitance of $R_0 = 3.36\,\Omega$ and $C = 2.54\,\mathrm{nF}$, respectively. In contrast to the filters in the main text, here the wire is wound as a 6 cm long and thin single layer coil to suppress parasitic capacitive couplings (due to the single layer design interlayer couplings are absent).

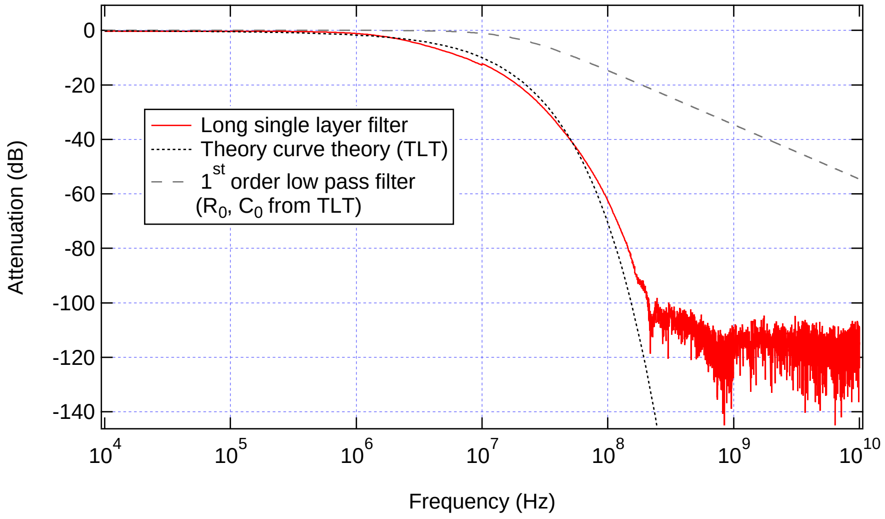


FIG. S1: Measured room temperature attenuation characteristics for a single layer microwave filter (no interlayer coupling) with $z = 1.51\,\mathrm{m}$ of copper wire (red data). A theory curve using eq. 1 and the parameters from Tab. I, is shown as dotted, black curve. In dashed grey, a standard first order low-pass filter ($R_0 = R_{\mathrm{tot}} z$ and $C_0 = Cz$ from theory curve) is shown for comparison.

The measured attenuation is in very good agreement with theoretical predictions for a 1.51 m long coax cable (black dashed line in Fig. S1) with inner and outer conductor made from copper and silver epoxy, respectively. We stress that the input parameters for the theory curve, given in Tab. I, arise from independently measured quantities and literature values that completely fix the attenuation profile without adjustable parameters. While the conductivity of copper $\sigma_{\mathrm{Cu}}$, the thickness $d_{\mathrm{epoxy}}$ of the epoxy layer have a minor infulence on the transmission profile (given the low conductivity $\sigma_{\mathrm{Ins.}}$ of pulyurethane, the shunt term is negligible), the other quantities affect it quite strongly.

We note that since $R_{\mathrm{tot}}$ is dominated by the outer conductor at high frequencies, a replace-

ment of the inner conductor with e.g. resistive wire, does not improve the filter performance, provided that the resistivity of the inner conductor stays well below that of silver epoxy. For the same reason, the transmission does not significantly alter at cryogenic temperatures, though the conductivity of the copper wire significantly increases (a residual resistance ratio of $RRR = 128$ was measured for the present wire, whereas $RRR \sim 3$ for the silver epoxy).

| | | |
|---|---|---|
| $D$ | $97 \pm 2\,\mu$m | measured ($D = 100\,\mu$m stated by the manufacturor[2]) |
| $d_{\text{Ins.}}$ | $8 \pm 2\,\mu$m | measured |
| $d_{\text{epoxy}}$ | $\approx 2\,$mm | cross section of the filter |
| $z$ | $1.51\,$m | measured |
| $\epsilon_{\text{Ins.}}$ | $4.6 \pm 1$ | chosen to match the measured capacitance with the above wire dimensions |
| $\sigma_{\text{Ins.}}$ | $< 9.3 \cdot 10^{-14}\,$S/m | measured |
| $\sigma_{\text{Cu}}$ | $5.95 \cdot 10^{7}\,$S/m | Ref. 4 |
| $\sigma_{\text{epoxy}}$ | $\geq 2 \cdot 10^{5}\,$S/m | Ref. 3 |

TABLE I: Material parameters and geometrical dimensions used for the theory curve shown in Fig. S1.

From eq. 2 the filter DC resistance $R_0 = (R_{\text{IC}}(\nu = 0) + R_{\text{OC}}(\nu = 0)) \cdot z \approx R_{\text{IC}}(\nu = 0) \cdot z$ can easily be calculated, $R_0 = 3.43 \pm 0.15\,\Omega$, in good agreement with the measured resistance of $3.36\,\Omega$.

To emphasize the filter performance, the theoretical attenuation profile for a standart first order low-pass filter with $R_0 = 3.36\,\Omega$ and $C_0 = 2.54\,$nF is shown in fig. S1 (dashed grey) in addition to the data and transmission line model.

* Electronic address: dominik.zumbuhl@unibas.ch

[1] David M. Pozar, Microwave Engineering, third edition, John Wiley & sons Inc. (2005)

[2] Insulated copper wire CUL 200/0.1, available at distrelec, *www.distrelec.ch*

[3] Datasheet for conductive silver epoxy E4110, available at EPO-TEK

[4] G. K. White and P. J. Meeson, Experimental techniques in low-temperature physics, Oxford University Press (2002).
